# Supplementary material for: LiDAR-MIMO: Efficient Uncertainty Estimation for LiDAR-based 3D Object Detection
Source: arXiv:2206.00214 source file (2022-06-01)
Supplement: Supplementary file 1 [file appendix.tex]

\section*{Appendix}

 We examine the mean average precision (mAP) of the PointPillars models trained on the CADC dataset in \ref{appendix:pp_cadc}. The ablation study over the batch size and input repetition for the MIMO-BEV PointPillars models trained on KITTI are in \ref{appendix:bs_and_ir}. We also perform ablation study on the number of heads as well as the capacity of the network for the MIMO-BEV PointPillars model trained on KITTI in \ref{appendix:extra_heads_wide}. Lastly,  we introduce and evaluate another input combination method for point clouds called MIMO-ID in \ref{appendix:mimo_id}.

\section{The mAP results for PointPillars models trained on the CADC dataset}
\label{appendix:pp_cadc}

\cref{tab:cadc_pp_map} contains the mAP results and detection partitions for the PointPillars models trained on the CADC dataset. The MIMO-BEV and MC dropout models perform worse than the Baseline, and both have equivalent mAP. However, the TP count for MIMO-BEV is higher than the count for MC dropout. Similarly to the MIMO-BEV SECOND model results in \cref{tab:cadc_second_map}, the FP\textsubscript{BG} count is lower than the baseline model for CADC.

\begin{table}[ht]
\small
\centering
\caption{The mAP and detection partitions for the PointPillars models trained on the CADC dataset. The bold indicates the best performing model for the associated metric.}
\label{tab:cadc_pp_map}
\begin{tabular}{ c|cccc }
 \Xhline{2\arrayrulewidth}
 \multirow{2}{*}{Model} & mAP & TP & FP\textsubscript{ML} & FP\textsubscript{BG} \\
 \cline{3-5}
  &  (\%) $\uparrow$ & \multicolumn{3}{c}{\tiny{Counts Per Partition}} \\
 \hline
  Baseline & 53.65 & 17483 & 8040 & 43661 \\
 \hline
  MC dropout & 50.49 & 16479 & 9057 & 34846 \\
  Ensemble & \textbf{56.53} & \textbf{17810} & \textbf{7225} & \textbf{19823} \\
  \hline
  MIMO-BEV & 50.47 & 17239 & 8087 & 33520 \\
 \Xhline{2\arrayrulewidth}
\end{tabular}
\end{table}

\section{The ablation study on batch size and input repetition for MIMO-BEV}
\label{appendix:bs_and_ir}

\cref{tab:kitti_pp_map_bs} and \cref{tab:kitti_pp_ue_bs} contain the results for MIMO-BEV models trained for different batch sizes and an input repetition of 0.0 With increasing the batch size (BS) the mAP decreases due to the increase of frame groupings (pairings) without matching frames. Note that frame pairings during training are produced by sampling a batch, then duplicating it and shuffling. Using this procedure with a batch size of 3 creates higher probability of matching frames than for batch size of 12. Due to the limited network capacity, fewer matching groupings result in a lower mAP. There are also fewer FP\textsubscript{BG} detections with a BS of 3 although the models with higher BSs have similar counts of FP\textsubscript{BG}. The scoring rules are best for the batch size of 9, although the scores are comparable.

\begin{table}[ht]
\small
\centering
\caption{The mAP and detection partitions for the PointPillars MIMO-BEV models trained over the KITTI dataset with increasing batch size (BS) and input repetition (IR) of 0. The bold indicates the best performing model for the associated metric.}
\label{tab:kitti_pp_map_bs}
\begin{tabular}{ cc|cccc }
 \Xhline{2\arrayrulewidth}
 \multirow{2}{*}{Model} & \multirow{2}{*}{BS} & mAP & TP & FP\textsubscript{ML} & FP\textsubscript{BG} \\
 \cline{4-6}
  & &  (\%) $\uparrow$ & \multicolumn{3}{c}{\tiny{Counts Per Partition}} \\
 \hline
  MIMO-BEV & 3 & \textbf{64.61} & \textbf{8332} & \textbf{3857} & \textbf{56988} \\
  MIMO-BEV & 6 & 64.01 & 8296 & 3904 & 61573 \\
  MIMO-BEV & 9 & 62.96 & 8243 & 3921 & 61571 \\
  MIMO-BEV & 12 & 61.86 & 8203 & 3928 & 59225 \\
 \Xhline{2\arrayrulewidth}
\end{tabular}
\end{table}

\begin{table*}[ht]
\footnotesize
\centering
\caption{Uncertainty evaluation for the PointPillars MIMO-BEV models trained on the KITTI dataset with increasing batch size (BS).}
\label{tab:kitti_pp_ue_bs}
\begin{tabular}{ cc|ccc|ccc|cc|cc|c|c }
 \Xhline{2\arrayrulewidth}
 \multirow{2}{*}{Model} & \multirow{2}{*}{BS} & \multicolumn{3}{c|}{NLL (Cls) $\downarrow$} & \multicolumn{3}{c|}{Brier Score $\downarrow$} & \multicolumn{2}{c|}{NLL (Reg) $\downarrow$} & \multicolumn{2}{c|}{Energy Score $\downarrow$} & MCE & CE \\
 \cline{3-12}
  & & TP & FP\textsubscript{ML} & FP\textsubscript{BG} & TP & FP\textsubscript{ML} & FP\textsubscript{BG} & TP & FP\textsubscript{ML} & TP & FP\textsubscript{ML} & (Cls) $\downarrow$ & (Reg) $\downarrow$ \\
 \hline
  MIMO-BEV & 3 & 0.3652 & 0.4445 & 0.9870 & 0.2011 & 0.2609 & 0.7633 & -5.0020 & -2.3396 & \textbf{0.4332} & 0.6704 & 0.2070 & \textbf{0.0642}\\
  MIMO-BEV & 6 & 0.3433 & 0.4193 & \textbf{0.9830} & 0.1860 & 0.2395 & \textbf{0.7630} & -4.8840 & \textbf{-2.3967} & 0.4453 & \textbf{0.6640} & \textbf{0.1902} & 0.0729\\
  MIMO-BEV & 9 & \textbf{0.3425} & \textbf{0.4184} & 0.9940 & \textbf{0.1855} & \textbf{0.2373} & 0.7654 & \textbf{-5.0472} & -1.8678 & 0.4597 & 0.6945 & 0.1984 & 0.0740\\
  MIMO-BEV & 12 & 0.3710 & 0.4381 & 1.0151 & 0.2070 & 0.2554 & 0.7795 & -4.9093 & -1.9856 & 0.4456 & 0.7099 & 0.1985 & 0.0748\\
 \Xhline{2\arrayrulewidth}
\end{tabular}
\end{table*}

\cref{tab:kitti_pp_map_ir} and \cref{tab:kitti_pp_ue_ir} contain the results for MIMO-BEV models trained with a batch size of 12 and increasing input repetitions of 0.0, 0.05, 0.1 and 0.2. A higher input repetition increases the percentage of frame groupings that contain the same frame. As already explained, with the larger batch size, the mAP is lowered due to the increased randomness of these frame groupings. This randomness is offset by having higher input repetition, however. Do to the limited capacity of the detectors, matching frame groupings need to be increased to improve mAP, but at the cost of subnetwork independence.

\begin{table*}[ht]
\footnotesize
\centering
\caption{Uncertainty evaluation for the PointPillars MIMO-BEV models trained on the KITTI dataset with a batch size of 12 and increasing input repetition (IR).}
\label{tab:kitti_pp_ue_ir}
\begin{tabular}{ cc|ccc|ccc|cc|cc|c|c }
 \Xhline{2\arrayrulewidth}
 \multirow{2}{*}{Model} & \multirow{2}{*}{IR} & \multicolumn{3}{c|}{NLL (Cls) $\downarrow$} & \multicolumn{3}{c|}{Brier Score $\downarrow$} & \multicolumn{2}{c|}{NLL (Reg) $\downarrow$} & \multicolumn{2}{c|}{Energy Score $\downarrow$} & MCE & CE \\
 \cline{3-12}
  & & TP & FP\textsubscript{ML} & FP\textsubscript{BG} & TP & FP\textsubscript{ML} & FP\textsubscript{BG} & TP & FP\textsubscript{ML} & TP & FP\textsubscript{ML} & (Cls) $\downarrow$ & (Reg) $\downarrow$ \\
 \hline
  MIMO-BEV & 0.00 & 0.3710 & 0.4381 & 1.0151 & 0.2070 & 0.2554 & 0.7795 & \textbf{-4.9093} & -1.9856 & 0.4456 & 0.7099 & 0.1985 & 0.0748 \\
  MIMO-BEV & 0.05 & \textbf{0.3612} & 0.4254 & 0.9912 & \textbf{0.1990} & 0.2444 & 0.7675 & -4.8154 & -2.0918 & 0.4736 & 0.7033 & 0.2000 & 0.0759 \\
  MIMO-BEV & 0.10 & 0.3647 & \textbf{0.4186} & 1.0288 & 0.2026 & \textbf{0.2420} & 0.7893 & -4.8043 & \textbf{-2.2328} & \textbf{0.4651} & \textbf{0.6888} & \textbf{0.1824} & 0.0716 \\
  MIMO-BEV & 0.20 & 0.3668 & 0.4241 & \textbf{0.9881} & 0.2024 & 0.2449 & \textbf{0.7639} & -4.6974 & -2.1661 & 0.4708 & 0.7014 & 0.2083 & \textbf{0.0676} \\
 \Xhline{2\arrayrulewidth}
\end{tabular}
\end{table*}

\begin{table}[ht]
\small
\centering
\caption{The mAP and detect partitions for the PointPillars MIMO-BEV models trained over the KITTI dataset with a batch size of 12 and input repetition (IR). The bold indicates the best performing model for the associated metric.}
\label{tab:kitti_pp_map_ir}
\begin{tabular}{ cc|cccc }
 \Xhline{2\arrayrulewidth}
 \multirow{2}{*}{Model} & \multirow{2}{*}{IR} & mAP & TP & FP\textsubscript{ML} & FP\textsubscript{BG} \\
 \cline{4-6}
  & &  (\%) $\uparrow$ & \multicolumn{3}{c}{\tiny{Counts Per Partition}} \\
 \hline
  MIMO-BEV & 0.0 & 61.86 & 8203 & 3928 & 59225 \\
  MIMO-BEV & 0.05 & 63.2 & 8234 & 4000 & 57918 \\
  MIMO-BEV & 0.1 & 63.87 & 8250 & 3953 & 56968 \\
  MIMO-BEV & 0.2 & \textbf{64.63} & \textbf{8297} & \textbf{3898} & \textbf{56279} \\
 \Xhline{2\arrayrulewidth}
\end{tabular}
\end{table}

\section{The ablation study on detection heads and network capacity for MIMO-BEV}
\label{appendix:extra_heads_wide}

To determine the effect of an increased number of detection heads on the network, we trained four MIMO-BEV models with a batch size of 3 and input repetition 0.0 for 120 epochs. For each model, we vary the number of detection heads being two or three as well as the regular and wide versions of the backbone. The wide version is created by doubling the number of filters for each VFE network and backbone component. By using the wide backbone, the network should be able to overcome capacity constraints and train with more detection heads~\cite{havasi2021training}.

\cref{tab:kitti_pp_map_wide} contains the average precision and detection results for the models. Our results show that there is a decrease of ~0.5\% mAP when adding an extra head to the network. This shows that the extra capacity of our network is not high enough to handle more detection heads. It also shows that switching the network to have the wide backbone causes a decrease in mAP of ~1\%. This could be due to the training time we set being equal for each model.

\cref{tab:kitti_pp_ue_wide} contains the results for the scoring rules and calibration errors for our models. In these results we can see that the wide model with 2 heads as well as the normal model with 3 heads perform best. Thus, adding either extra capacity or an extra head to the regular two-head variant slightly improved the uncertainty results, i.e., lower scores. 

\begin{table}[ht]
\footnotesize
\centering
\caption{The mAP and detect partitions for the PointPillars MIMO-BEV models trained over the KITTI dataset with increased detection heads as well as network capacity. The bold indicates the best performing model for the associated metric.}
\label{tab:kitti_pp_map_wide}
\begin{tabular}{ ccc|cccc }
 \Xhline{2\arrayrulewidth}
 \multirow{2}{*}{Model} & \multirow{2}{*}{Heads} & \multirow{2}{*}{Wide} & mAP & TP & FP\textsubscript{ML} & FP\textsubscript{BG} \\
 \cline{4-6}
  & & &  (\%) $\uparrow$ & \multicolumn{3}{c}{\tiny{Counts Per Partition}} \\
 \hline
  MIMO-BEV & 2 & & \textbf{64.61} & \textbf{8332} & 3857 & 56988 \\
  MIMO-BEV & 2 & \checkmark & 63.57 & 8303 & \textbf{3796} & \textbf{52159} \\
  MIMO-BEV & 3 & & 64.14 & 8300 & 3969 & 72885 \\
  MIMO-BEV & 3 & \checkmark & 63.07 & 8295 & 3866 & 58678 \\
 \Xhline{2\arrayrulewidth}
\end{tabular}
\end{table}

\section{MIMO-ID}
\label{appendix:mimo_id}

\subsection{Input combination}
For the MIMO-ID variant, we combine the point clouds before the VFE network and add an additional feature to each point in the point cloud to separate the point clouds from one another. \Cref{f:mimo_id_training} depicts the MIMO-ID architecture for training. In step 1, one point cloud for each detection head is individually voxelized. In step 2, a head ID feature is added to each point in the voxels. The final step is to merge the voxels as the input to the VFE network. This combination method of adding head IDs allows the detection heads to focus on features from their corresponding point cloud. It also ensures that the voxels are filled evenly by all inputs. During testing, we found that the voxel merging strategy was slow and took a different approach to slightly increase the data processing speed. We follow the steps in \cref{f:mimo_id_testing}. A single point cloud is duplicated for each detection head in step 1, followed by the additional head ID features being added to the points. In step 2 we merge the point clouds into a single cloud by simply concatenating their arrays. In step 3 the point cloud must be shuffled. This is to resolve the problem of voxels being filled from only the first point cloud in the point array. In the final step, the point cloud is voxelized and send to the VFE network. During training and testing, the maximum number of points per voxel must be multiplied by the number of detection heads, compared to the original implementation.

\subsection{The inference time}
In \cref{tab:mimo_id_timing} we show the inference timing results for MIMO-ID along with MIMO-BEV for comparison. Despite our attempts to decrease the data processing time during testing, MIMO-ID requires an additional 30~{ms}. The larger voxels also cause an increase in time for the VFE network, although it is only a 1~{ms} increase.

\begin{table}[ht]
\scriptsize
\centering
\caption{The inference time (in \textit{ms}) for the PointPillars MIMO-ID and MIMO-BEV models trained on the KITTI dataset}
\label{tab:mimo_id_timing}
\begin{tabular}{ c|ccccc } 
 \Xhline{2\arrayrulewidth}
\multirow{2}{*}{Model} & \multirow{2}{*}{\begin{tabular}[c]{@{}c@{}}\# Fwd\\ Passes\end{tabular}} & \begin{tabular}[c]{@{}c@{}}Data\\ Processing\end{tabular} & VFE & \begin{tabular}[c]{@{}c@{}}Backbone +\\ Heads \end{tabular} & \multirow{2}{*}{\begin{tabular}[c]{@{}c@{}}Total\\ Time $\downarrow$\end{tabular}} \\ \cline{3-5}
 &  & \multicolumn{3}{c}{\tiny{1 Fwd Pass}} &  \\
 \hline
 MIMO-BEV & 1 & 16 & 4 & 25 & \textbf{45} \\
 MIMO-ID & 1 & 46 & 5 & 25 & 76 \\
 \Xhline{2\arrayrulewidth}
\end{tabular}
\end{table}

\subsection{The mAP and detection partitions}
In \cref{tab:mimo_id_map} we show the mAP and detection partition counts for the MIMO-ID models trained on the KITTI dataset. The MIMO-ID PointPillars model trained on KITTI performs only 0.32\% worse than the MIMO-BEV model. The MIMO-ID SECOND model performs better than the MIMO-BEV version by 0.72\%. In both MIMO-ID models, the FP\textsubscript{BG} is lower showing that point cloud combination may be better at removing FP\textsubscript{BG} detections. The number of  FP\textsubscript{BG} detections is equivalent to or lower than the baseline models.

\begin{table}[ht]
\small
\centering
\caption{The mAP and detection partitions for the MIMO models trained over the KITTI dataset}
\label{tab:mimo_id_map}
\begin{tabular}{ c|cccc }
 \Xhline{2\arrayrulewidth}
 \multirow{2}{*}{Model} & mAP & TP & FP\textsubscript{ML} & FP\textsubscript{BG} \\
 \cline{3-5}
  &  (\%) $\uparrow$ & \multicolumn{3}{c}{\tiny{Counts Per Partition}} \\
 \hline
  MIMO-BEV (PP) & 64.61 & 8332 & 3857 & 56988 \\
  MIMO-ID (PP) & 64.29 & 8250 & 3905 & 53593 \\
  \hline
  MIMO-BEV (SC) & 65.45 & 8534 & 3581 & 44113 \\
  MIMO-ID (SC) & \textbf{66.17} & \textbf{8586} & \textbf{3497} & \textbf{36509} \\
 \Xhline{2\arrayrulewidth}
\end{tabular}
\end{table}

\begin{figure*}[ht]
\centering
\includegraphics[width=0.7\textwidth]{images/mimo_id_training.pdf}
\caption{Voxel merging during training for MIMO-ID with two inputs}
\label{f:mimo_id_training}
\end{figure*}

\begin{figure*}[ht]
\centering
\includegraphics[width=1.0\textwidth]{images/mimo_id_testing.pdf}
\caption{Point cloud merging during training for MIMO-ID with two inputs}
\label{f:mimo_id_testing}
\end{figure*}

\begin{table*}[ht]
\scriptsize
\centering
\caption{Uncertainty evaluation for the PointPillars MIMO-BEV models trained on the KITTI dataset with increased detection heads as well as network capacity.}
\label{tab:kitti_pp_ue_wide}
\begin{tabular}{ ccc|ccc|ccc|cc|cc|c|c }
 \Xhline{2\arrayrulewidth}
 \multirow{2}{*}{Model} & \multirow{2}{*}{Heads} & \multirow{2}{*}{Wide} & \multicolumn{3}{c|}{NLL (Cls) $\downarrow$} & \multicolumn{3}{c|}{Brier Score $\downarrow$} & \multicolumn{2}{c|}{NLL (Reg) $\downarrow$} & \multicolumn{2}{c|}{Energy Score $\downarrow$} & MCE & CE \\
 \cline{4-13}
  & & & TP & FP\textsubscript{ML} & FP\textsubscript{BG} & TP & FP\textsubscript{ML} & FP\textsubscript{BG} & TP & FP\textsubscript{ML} & TP & FP\textsubscript{ML} & (Cls) $\downarrow$ & (Reg) $\downarrow$ \\
 \hline
  MIMO-BEV & 2 & & 0.3652 & 0.4445 & 0.9870 & 0.2011 & 0.2609 & 0.7633 & -5.0020 & -2.3396 & 0.4332 & 0.6704 & 0.2070 & 0.0642 \\
  MIMO-BEV & 2 & \checkmark & 0.3591 & \textbf{0.4172} & 1.0152 & \textbf{0.1953} & \textbf{0.2395} & 0.7812 & \textbf{-5.0643} & \textbf{-2.5511} & 0.4511 & \textbf{0.6557} & 0.2041 & \textbf{0.0577} \\
  MIMO-BEV & 3 & & \textbf{0.3590} & 0.4602 & \textbf{0.9435} & 0.2001 & 0.2713 & \textbf{0.7280} & -4.8333 & -1.9523 & 0.4722 & 0.7044 & \textbf{0.1859} & 0.0727 \\
  MIMO-BEV & 3 & \checkmark & 0.3728 & 0.4337 & 0.9827 & 0.2072 & 0.2513 & 0.7595 & -4.9897 & -2.1837 & \textbf{0.4060} & 0.6668 & 0.2014 & 0.0588 \\
 \Xhline{2\arrayrulewidth}
\end{tabular}
\end{table*}

\begin{table*}[ht]
\footnotesize
\centering
\caption{Uncertainty evaluation for the MIMO models trained over the KITTI dataset}
\label{tab:mimo_id_ue}
\begin{tabular}{ c|ccc|ccc|cc|cc|c|c }
 \Xhline{2\arrayrulewidth}
 \multirow{2}{*}{Model} & \multicolumn{3}{c|}{NLL (Cls) $\downarrow$} & \multicolumn{3}{c|}{Brier Score $\downarrow$} & \multicolumn{2}{c|}{NLL (Reg) $\downarrow$} & \multicolumn{2}{c|}{Energy Score $\downarrow$} & MCE & CE \\
 \cline{2-11}
  & TP & FP\textsubscript{ML} & FP\textsubscript{BG} & TP & FP\textsubscript{ML} & FP\textsubscript{BG} & TP & FP\textsubscript{ML} & TP & FP\textsubscript{ML} & (Cls) $\downarrow$ & (Reg) $\downarrow$ \\
 \hline
  MIMO-BEV (PP) & \textbf{0.3652} & 0.4445 & 0.9870 & \textbf{0.2011} & 0.2609 & 0.7633 & -5.0020 & -2.3396 & 0.4332 & 0.6704 & 0.207 & 0.0642 \\
  MIMO-ID (PP) & 0.3762 & \textbf{0.4389} & 1.0044 & 0.2115 & \textbf{0.2572} & 0.772 & -5.0557 & \textbf{-2.3631} & 0.4539 & 0.7188 & 0.1987 & \textbf{0.0625} \\
  \hline
  MIMO-BEV (SC) & 0.4185 & 0.5691 & 0.7290 & 0.2567 & 0.3692 & 0.5395 & -4.3107 & -0.1172 & 0.3688 & 0.8665 & \textbf{0.1845} & 0.0652 \\
  MIMO-ID (SC) & 0.8050 & 1.0483 & \textbf{0.4724} & 0.6018 & 0.7147 & \textbf{0.3016} & \textbf{-5.5405} & -2.065 & \textbf{0.2991} & \textbf{0.5985} & 0.1876 & 0.0631 \\
 \Xhline{2\arrayrulewidth}
\end{tabular}
\end{table*}

\subsection{Uncertainty evaluation metrics}
The uncertainty results for the MIMO-ID PointPillars and SECOND models trained on the KITTI dataset are shown in \cref{tab:mimo_id_ue}. The TP and FP\textsubscript{ML} scores for classification are much higher for MIMO-ID (SC) and are outliers compared to the other models. The MIMO-ID (SC) model outputs predictions with much lower confidence compared to the other models. For the regression scores, the MIMO-ID (SC) model outperforms the PP model as expected based on lower regression uncertainty scores for SC models  by comparing in \cref{tab:kitti_pp_ue} and \cref{tab:kitti_second_ue}. It also performs similarly to the other results for SECOND models.
